# Supplementary material for: ClothesNet: An Information-Rich 3D Garment Model Repository with Simulated Clothes Environment
Source: arXiv:2308.09987 source file (2023-08-19)
Supplement: Supplementary file 1 [file supp.tex]

\section{Dressing}
In the dressing task, we load an articulated human model into the scene as shown in Fig~\ref{fig:dress}. The human model has the spherical joint on the left/right shoulder, the revolute joint on the left/right elbow. To order to get the human model dressed, we need to control the human model's arms and the garment simultaneously. The action space thus contains the human model's arm joint values and the control points defined on the garment. In the dressing task, we define the two control points on the collar's left and right sides.

The dressing task is a long-horizon task, containing multiple stages where the human model needs to change the arm poses such that the garment can be pulled toward a reasonable shape. We show a heuristic trajectory in the video. Fig~\ref{fig:dress} also shows the procedures. We have not successfully trained the agent to accomplish the task using existing reinforcement learning algorithms (TD3~\cite{fujimoto2018addressing} and SAC~\cite{haarnoja2018soft}), mainly due to the task's complexity and difficulty.
The dressing task could be formulated as either an imitation learning/learning from visual demonstration task or a long-horizon reinforcement learning/planning task. A video is also available in the zip file.
\begin{figure*}[thb!]
\centering
 \includegraphics[width=0.99\linewidth]{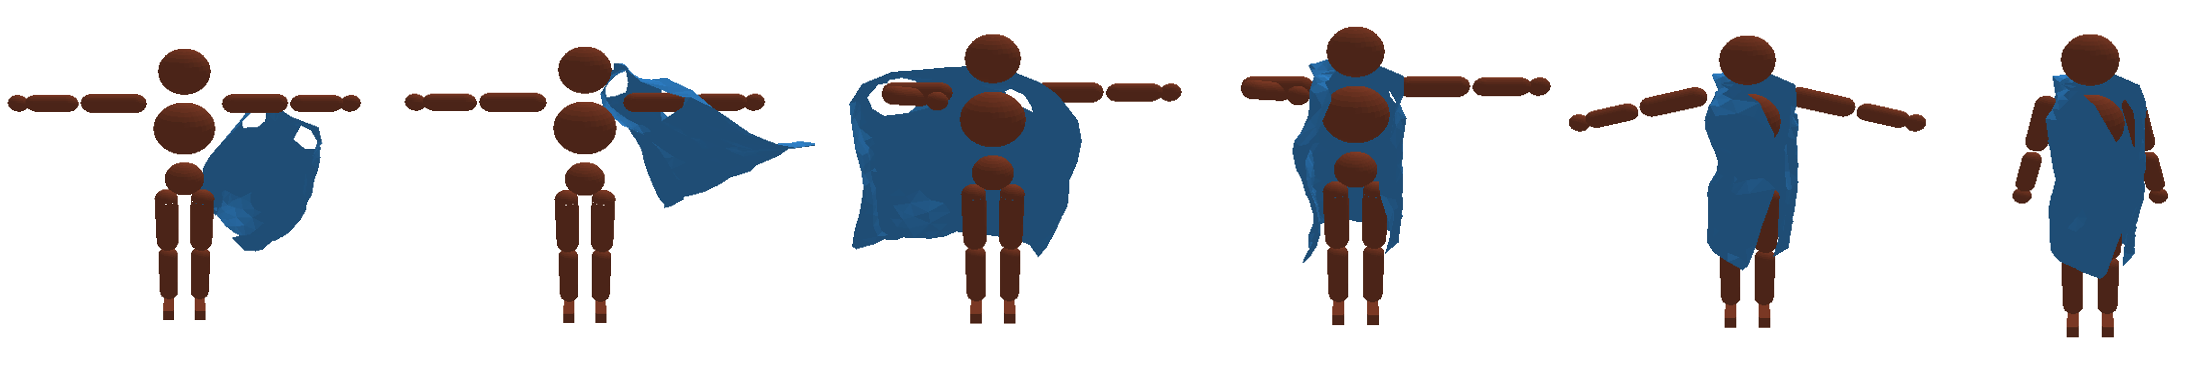}
 \caption{Dressing Task}
\label{fig:dress}
\end{figure*}

\section{Folding, Hanging, Rearranging Task}
The video for each task is available in the zip file. We have selected the control points and key points on the clothes based on human knowledge, which might be more than sufficient to accomplish the tasks. The states used in our RL experiments are the positions and velocities of key vertices on the clothes. We also specify the \emph{target} positions/velocities of key vertices when the clothes reach the desired positions/shapes.
The reward/loss functions are derived based on the differences between the \emph{target} and \emph{current} positions/vertices of key vertices in the process.

There are various alternative definitions. For example, instead of using the key vertices of the clothes, the images of the clothes captured by a RGB/RGBD camera are also feasible to be used as the state. It might take more training steps for the agent to accomplish the tasks. Based on our cloth simulation, the users could adopt the most suitable formulations to satisfy their task requirements.

Another interesting question to explore is what are the most effective control points to perform various tasks. For example, only two points might be already enough to accomplish the folding task, as we demonstrated in the real robot experiment. But how to identify/locate the two control points remains an open-ended problem.

\section{Differentiable simulation and coupling with articulated rigid bodies}
\begin{figure*}[thb!]
\centering
 \includegraphics[width=0.99\linewidth]{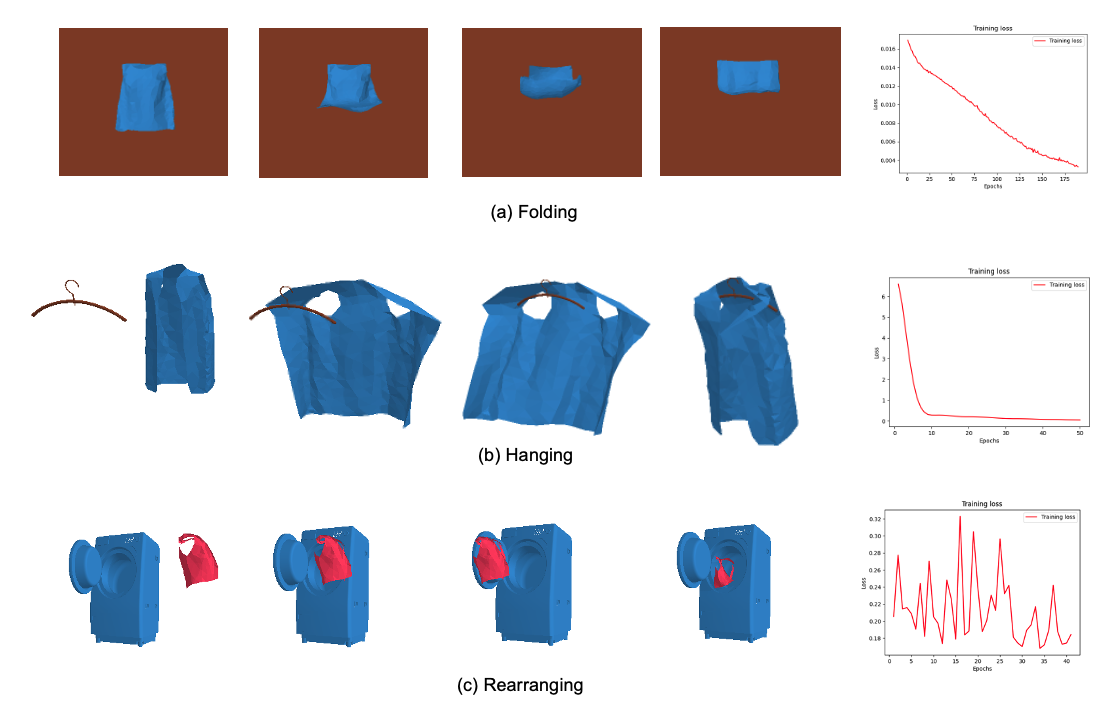}
 \caption{Fig(a) shows the folding task and Fig(b) shows the hanging task. Fig(c) reflects the rearranging task.}
\label{fig:diffloss}
\end{figure*}

Our simulated clothes environments provide the differentiation operations to calculate the gradients information, which enhances the learning process. With the loss function specified in each task, we could derive the gradient of each task's loss value with respect to the action and then update the action according to the gradient. 

We roll out an action trajectory defined as $\vec{a}$. Each action trajectory results in a final state associated with a loss or reward. We define the reward as $r$. Inside the differentiable cloth simulation, we have access to the $\frac{\partial{r}}{\partial{\vec{a}}}$. The action is then updated following the gradient descent fashion as below
\begin{equation}
\vec{a} = \vec{a} + \lambda \frac{\partial{r}}{\partial{\vec{a}}}
\end{equation}, where $\lambda$ is the updating parameter.
We visualize each task's manipulation process and the corresponding loss curve shown in Fig.~\ref{fig:diffloss}. For each row in Fig.~\ref{fig:diffloss}, the four left images reflect the sequence of accomplishing each task, and the rightmost image is the loss curve of optimization epochs. We can achieve each task within a few hundred epochs. The loss curves in the rearranging task are not smooth. One possible explanation is that in the process of putting the clothes inside the washing machine, there are heavy collisions and contact between the clothes and the washing machine. The heavy collision response and contact introduce non-smoothness in the optimization procedures.

Compared to the classic reinforcement learning approaches, the gradients collected from the differentiable cloth simulation significantly reduce the training steps. It indicates that the gradients, which incorporate the clothes and articulated rigid bodies' dynamics, are very informative in order to accomplish the task.

In addition, our simulation supports the differentiable coupling between clothes and articulated rigid bodies. Such differentiable coupling is useful for tasks requiring the interaction between clothes and the articulated rigid bodies, for example, in the \emph{dressing} task as shown in Fig~\ref{fig:dress}. The action space in \emph{dressing} contains both the clothes and the human model's arm. The differentiable coupling provides the gradient information of both the clothes and articulated rigid bodies' states and actions, which are probably useful to develop efficient learning algorithms.

%We report the different setting of these four tasks, including different states and action descriptions, in our supplementary material.

\section{Real-world Folding}
For the real experiment. A t-shirt is laid flat on the table in front of MOVO. We first extract the t-shirt pointcloud by applying color segmentation on the RGB image and recover the point position from the aligned masked depth image with known camera intrinsic and extrinsic. The pointcloud is passed for further outlier removal by detecting the number of neighbors of a point given a radius of 2.5cm and removing those that have less than 20 neighbor points. The de-noised pointcloud is then down-sampled to 2048 points and passed to Skeleton Merger model for keypoint prediction. 

%To enable more robust keypoint prediction on flat configuration, we additionally generated 3k flattened meshes from the existing meshes in two manners and retrained the model. Half of the data is generated by directly flattening the mesh. We shrink the z distance of a vertex to its mean value to 0.1 $\pm$ 0.005 of the original value: \[z^{'} = z_{mean} + random(0.095, 0.105) * (z - z_{mean})\]
%\begin{figure}[h!]
%\centering
%\subfigure{
% \begin{minipage}[t]{0.42\linewidth}
%    \centering
%    \includegraphics[width=\textwidth]{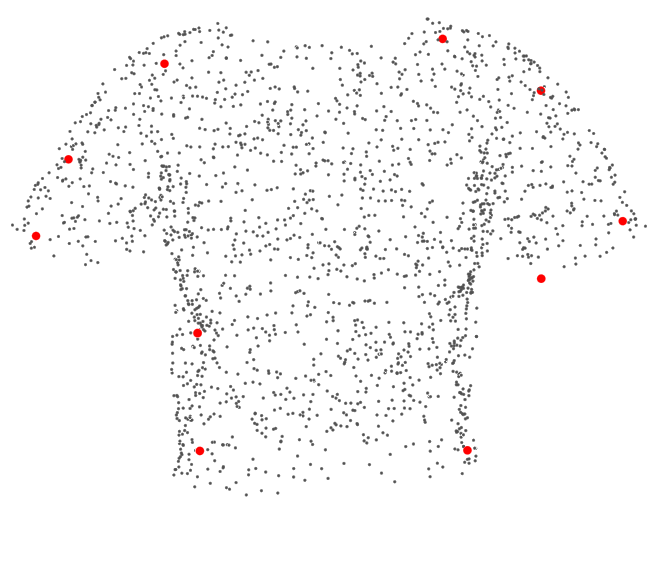}
%    \label{fig: flatten train data}
%    \end{minipage}}
%\subfigure{
% \begin{minipage}[t]{0.4\linewidth}
%    \centering
%    \includegraphics[width=\textwidth]{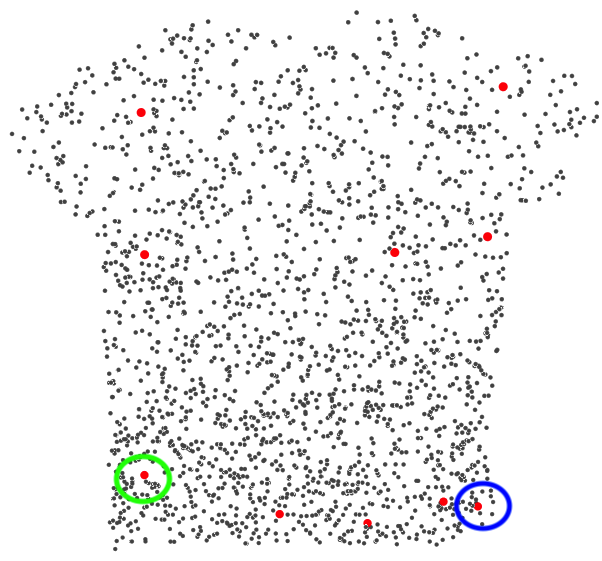}
%    \label{fig: flatten white tshirt }
%   \end{minipage}}
%\caption{(Left): flattened training mesh; (Right): keypoint prediction on the real t-shirt. The identified grasp points are circled in green and blue}
%\label{fig:real_keypoint}
%\end{figure}
\begin{figure}[h!]
\centering
 \begin{minipage}[t]{0.42\linewidth}
    \centering
\includegraphics[width=\textwidth]{imgs/flat_keypoint_white_tshirt.png}
    \label{fig: flatten train data}
    \end{minipage}
\caption{keypoint prediction on the real t-shirt. The identified grasp points are circled in green and blue}
\label{fig:real_keypoint}
\end{figure}

\begin{figure}[h!]
\centering
 \includegraphics[width=0.87\linewidth]{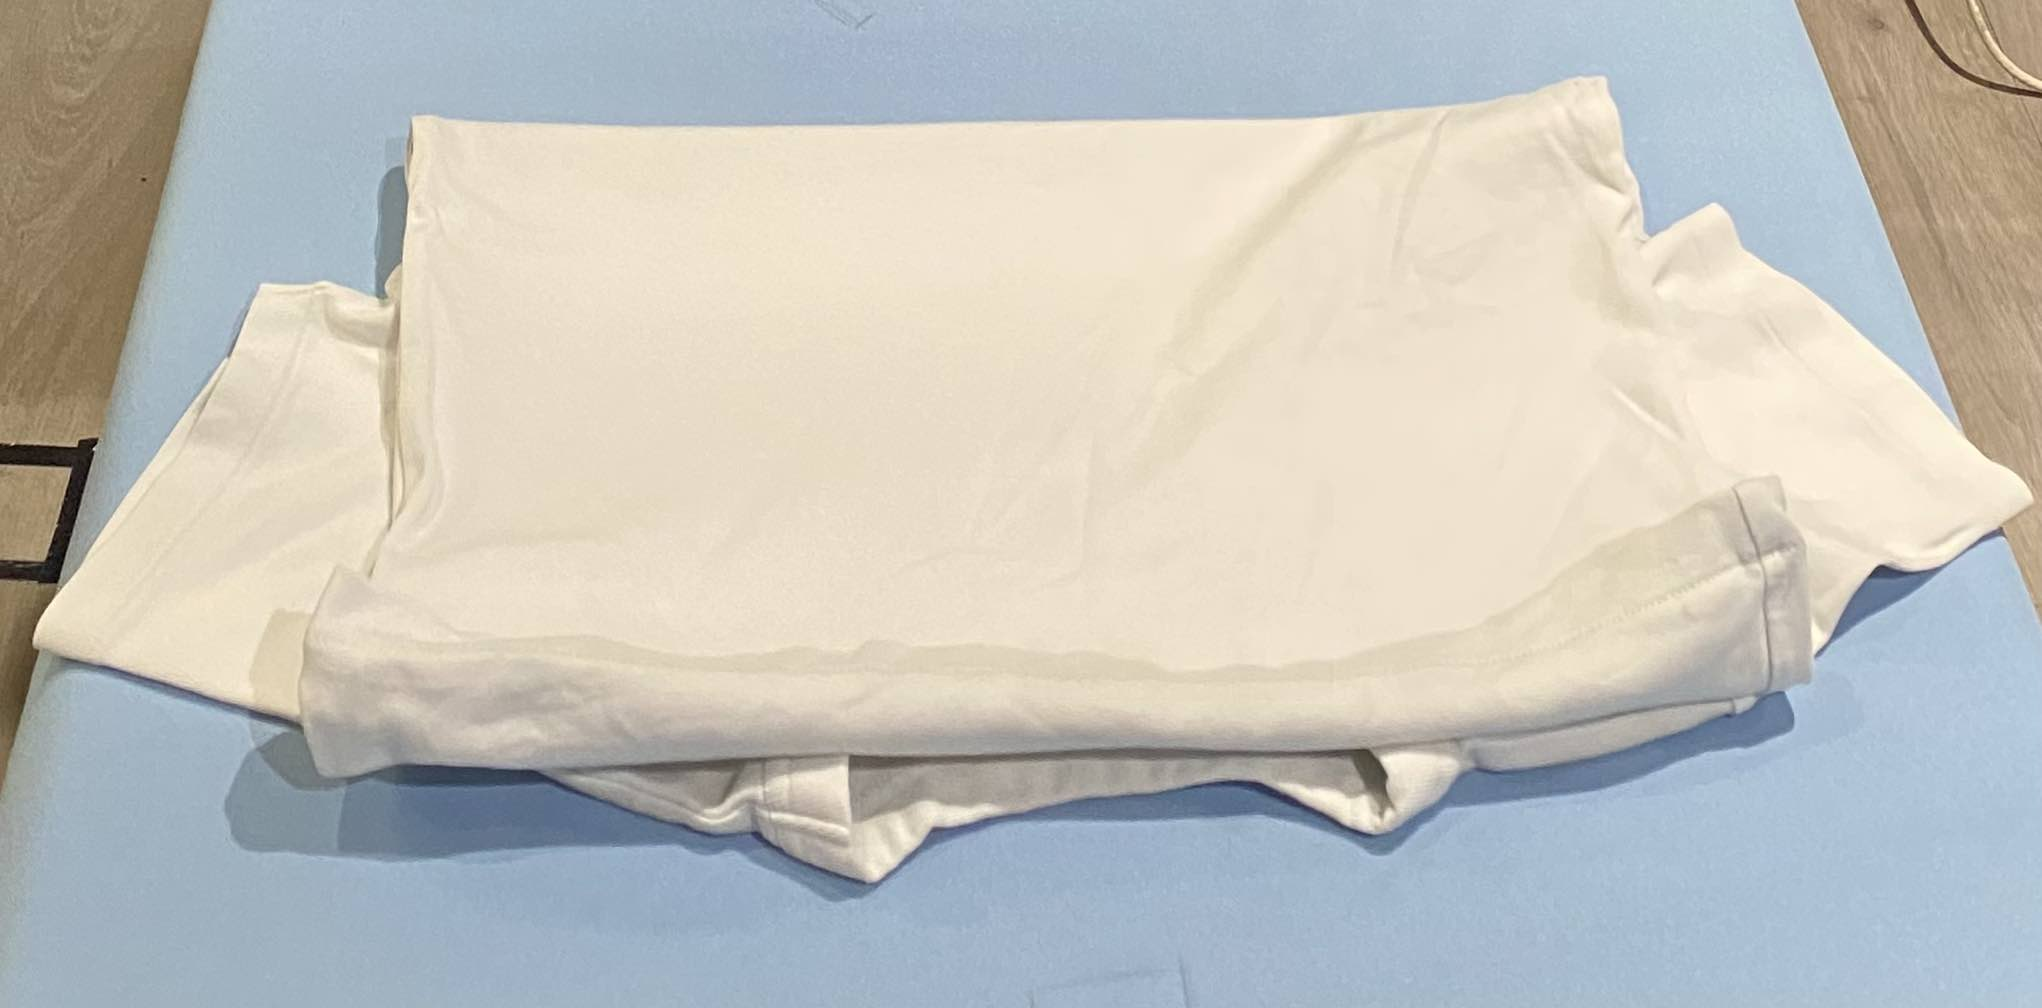}
 \caption{Folded t-shirt.}
\label{fig:foldedclothes}
\end{figure}

%We also simulated the clothes falling in flat under gravity onto a surface in physics simulation and generated the other half pointcloud from single view RGB-D similar to the real setup. The mesh and keypoint prediction is visualized in Figure ~\ref{fig:real_keypoint}. More detailed training samples can be checked in Figure~\ref{fig:shrink}.

For folding, We first identify the two grasp points from the predicted keypoints then apply a heuristic-based folding policy. %A minimal fitting bounding box on the xy-plane is calculated and we extracted four keypoints that are nearest to its corners. 
Two keypoints on the bottom were selected as the grasp points to grasp vertically. The folding is done by moving the grasped two points to the top two corner keypoints. As the joint limit might exceed when the t-shirt is long, both arms will move up first then move forward which is similar to human folding. The complete folding video of MOVO is also included in the supplementary material. 

% \begin{figure*}[h!]
%   \begin{center}
%    \includegraphics[width=0.87\linewidth]{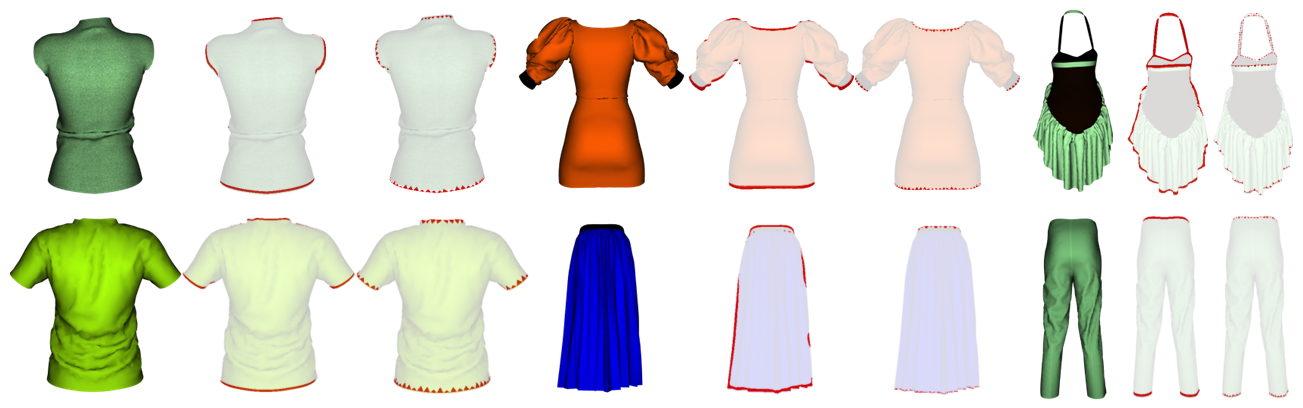}
%   \end{center}
%   \caption{We visualize some examples of our Unet experiment. For each instance pair, the leftmost subfigure shows the clothes. The middle figure is the predicted 2d boundary segmentation result highlighted as red lines, and the rightmost subfigure indicates the ground-truth 2d boundary segmentation annotations highlighted as red lines. For a better representation of boundary red lines, we transparency the garment pictures.}
% \label{fig:2d_seg}
% \end{figure*}

%\begin{figure*}[th!]
%  \begin{center}
%   \includegraphics[width=0.87\linewidth]{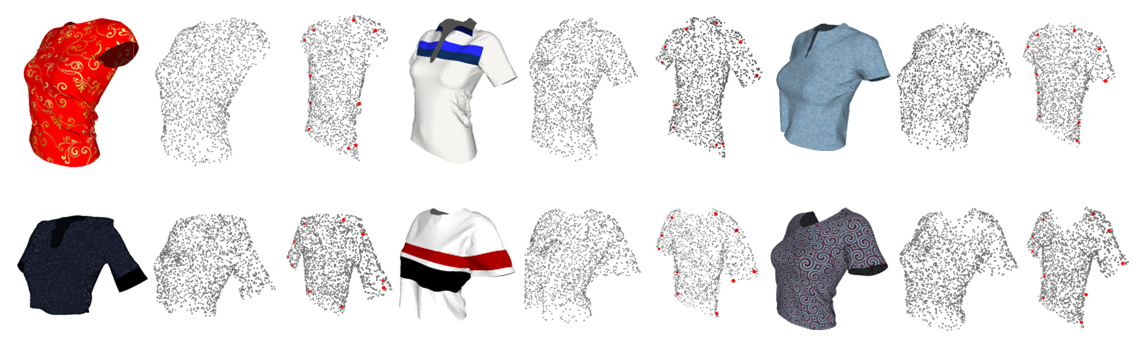}
%  \end{center}
%  \caption{We visualize some t-shirt instances of this shrinking process. For each instance pair, the leftmost subfigure shows the clothes. The middle figure is the downsampled point cloud before shrinking, and the rightmost subfigure indicates downsampled point cloud after shrinking at the same viewpoint with predicted keypoints highlighted as red points.}
%\label{fig:shrink}
%\end{figure*}

\section{Differentiable Cloth Simulation}
We provide documentation to explain our differentiable cloth simulation with intersection-free frictional contact and differentiable coupling with articulated rigid bodies. The documentation is
 a separate pdf inside the zip file.
